# Supplementary material for: SimPLE: Similar Pseudo Label Exploitation for Semi-Supervised Classification
Source: arXiv:2103.16725 source file (2022-06-29)
Supplement: Supplementary file 1 [file ablation-full.tex]

\begin{table*}[!ht]
    \centering
    \begin{tabularx}{\textwidth}{ X|X|c|c|c|c|c }
        \hline
        \multicolumn{7}{c}{Ablations: CIFAR-100} \\
        \hline
        Ablation & Augmentation Type & $\lambda_{\mathcal{P}}$ & $\tau_c$ & $\tau_s$ & K & 10000 labels \\
        \hline\hline
        \textbf{SimPLE} & RandAugment & 150 & 0.95 & 0.9 & 2 &70.82\% \\
        % \textbf{SimPLE} & RandAugment & 150 & 0.95 & 0.9 & \underline{7} &\textbf{73.04}\% \\
        % w/o Pair Loss & RandAugment & \underline{0} & 0.95 & 0.9 & 2 & 69.07\% \\
        % w/o RandAugment & \underline{fixed} & 150 & 0.95 & 0.9 & 2 & 67.91\% \\
        % w/o RandAugment, w/o Pair Loss & \underline{fixed} & \underline{0} & 0.95 & 0.9 & 2 & 67.41\% \\
        \hline

        % $\tau_c$ = 0.75 & RandAugment & 150 & \underline{0.75} & 0.9 & 2 & 71.96\% \\
        % $\tau_s$ = 0.7 & RandAugment & 150 & 0.95 & \underline{0.7} & 2 & 70.85\%  \\
        % $\tau_c$ = 0.75, $\tau_s$ = 0.7 & RandAugment & 150 & \underline{0.75} & \underline{0.7} & 2 & 71.48\% \\
        $\tau_c$ = 0.55, $\tau_s$ = 0.5 & RandAugment & 150 & \underline{0.55} & \underline{0.5} & 2 & 71.25\% \\
        \hline

        $\lambda_{\mathcal{P}}$ = 1 & RandAugment & \underline{1} & 0.95 & 0.9 & 2 & 69.04\% \\
        % $\lambda_{\mathcal{P}}$ = 50 & RandAugment & \underline{50} & 0.95 & 0.9 & 2 & 71.34\% \\
        $\lambda_{\mathcal{P}}$ = 200 & RandAugment & \underline{200} & 0.95 & 0.9 & 2 & 70.92\% \\
        % $\lambda_{\mathcal{P}}$ = 250 & RandAugment & \underline{250} & 0.95 & 0.9 & 2 & 71.42\% \\
        \hline
    \end{tabularx}
    \caption{Additional ablation study on CIFAR-100. All experiments using WRN 28-2}
    \label{table:ablation-full}
\end{table*}
